# Supplementary material for: CGD: Constraint-Guided Diffusion Policies for UAV Trajectory Planning
Source: arXiv:2405.01758 source file (2024-05-02)
Supplement: Supplementary file 1 [file supplementary-material.tex]

%!TEX root=../main.tex
%
\section*{Supplementary Material}%\label{sec:supMaterial}
\noindent\textbf{Video}: \href{https://youtu.be/W73p42XRcaQ}{https://youtu.be/W73p42XRcaQ} \\
\textbf{Code}: \href{https://github.com/mit-acl/puma}{https://github.com/mit-acl/puma}
